# Supplementary material for: DataFlow-Harness: A Grounded Code-Agent Platform for Constructing Editable LLM Data Pipelines
Source: arXiv:2607.16617 source file (2026-07-24)
Supplement: Supplementary file 1 [file x_appendix.tex]

\section{Author Contributions}

\newcommand{\ProjectSupervisor}{\textcolor{purple!70!black}{\textit{Project Supervisor}}}
\newcommand{\CorrespondingAuthor}{\textcolor{orange!80!black}{\textit{Corresponding Author}}}

\begin{itemize}
    \item Wentao Zhang: \CorrespondingAuthor, \ProjectSupervisor; manuscript writing and project supervision.
\end{itemize}
